# Supplementary material for: Contextual Personalized Re-Ranking of Music Recommendations through Audio Features
Source: arXiv:2009.02782 source file (2020-09-06)
Supplement: Supplementary file 1 [file A.tex]

\section{Re-rank Results}\label{appendix:A}
The three tables below show the results when re-ranking the top 50 recommended songs for the BPR, US-BPR and CAMF\_ICS initial recommendation algorithms respectively. Each show a selection of 5 $\lambda$ values and its corresponding Prec@10 and MAP@10 scores for the initial, global model based and personalized model based recommendations.

\begin{table}[ht]
\captionsetup{justification=centering} \scalebox{0.85}{\begin{tabular}{|l|l|l|l|l|l|l|l|l|l|l|}
\hline
List size	& \multicolumn{10}{c|}{50} \\ \hline
\textbf{}	& \multicolumn{2}{c|}{$\lambda$ = 0.2}	& \multicolumn{2}{c|}{$\lambda$ = 0.4}	& \multicolumn{2}{c|}{$\lambda$ = 0.6}	& \multicolumn{2}{c|}{$\lambda$ = 0.8}	& \multicolumn{2}{c|}{$\lambda$ = 1.0} \\ \hline
\textbf{}	& Prec@10	& MAP@10	& Prec@10	& MAP@10	& Prec@10	& MAP@10	& Prec@10	& MAP@10	& Prec@10	& MAP@10	 \\ \hline
Initial	& 0.02684	& 0.0116	& 0.02684	& 0.0116	& 0.02684	& 0.0116	& 0.02684	& 0.0116	& 0.02684	& 0.0116	 \\ \hline
\begin{tabular}[c]{@{}l@{}}Re-ranked\\ Global\end{tabular}	& \textbf{0.02614}	& \textbf{0.01116}	& 0.02491	& 0.01067	& 0.02475	& 0.01036	& 0.02386	& 0.01003	& 0.0233	& 0.00979	 \\ \hline
\begin{tabular}[c]{@{}l@{}}Re-ranked\\ Personal\end{tabular}	& 0.02742	& 0.01229	& 0.02705	& \textbf{0.0123}	& \textbf{0.02749}	& 0.01198	& 0.02633	& 0.01187	& 0.02609	& 0.01178	 \\ \hline
\end{tabular}}
\caption*{Re-rank results for the \textbf{BPR} initial recommendation for both global and personal model, evaluated over the \textbf{top 10} songs in the recommendation list consisting of the top \textbf{50 songs} using the \textit{time of day} dimension.}\label{tab:res-BPR-50-10}
\end{table}

\begin{table}[ht]
\captionsetup{justification=centering} \scalebox{0.85}{\begin{tabular}{|l|l|l|l|l|l|l|l|l|l|l|}
\hline
List size	& \multicolumn{10}{c|}{50} \\ \hline
\textbf{}	& \multicolumn{2}{c|}{$\lambda$ = 0.2}	& \multicolumn{2}{c|}{$\lambda$ = 0.4}	& \multicolumn{2}{c|}{$\lambda$ = 0.6}	& \multicolumn{2}{c|}{$\lambda$ = 0.8}	& \multicolumn{2}{c|}{$\lambda$ = 1.0} \\ \hline
\textbf{}	& Prec@10	& MAP@10	& Prec@10	& MAP@10	& Prec@10	& MAP@10	& Prec@10	& MAP@10	& Prec@10	& MAP@10	 \\ \hline
Initial	& 0.02508	& 0.01125	& 0.02508	& 0.01125	& 0.02508	& 0.01125	& 0.02508	& 0.01125	& 0.02508	& 0.01125	 \\ \hline
\begin{tabular}[c]{@{}l@{}}Re-ranked\\ Global\end{tabular}	& \textbf{0.02545}	& \textbf{0.01077}	& 0.0243	& 0.01003	& 0.02317	& 0.00974	& 0.02268	& 0.00947	& 0.02189	& 0.00893	 \\ \hline
\begin{tabular}[c]{@{}l@{}}Re-ranked\\ Personal\end{tabular}	& 0.02633	& 0.01198	& 0.02601	& 0.01244	& \textbf{0.02666}	& \textbf{0.01252}	& 0.02612	& 0.01251	& 0.02566	& 0.01201	 \\ \hline
\end{tabular}}
\caption*{Re-rank results for the \textbf{UserSplitting-BPR} initial recommendation for both global and personal model, evaluated over the \textbf{top 10} songs in the recommendation list consisting of the top \textbf{50 songs} using the \textit{time of day} dimension.}\label{tab:res-UserSplitting-BPR-50-10}
\end{table}

\begin{table}[ht]
\captionsetup{justification=centering} \scalebox{0.85}{\begin{tabular}{|l|l|l|l|l|l|l|l|l|l|l|}
\hline
List size	& \multicolumn{10}{c|}{50} \\ \hline
\textbf{}	& \multicolumn{2}{c|}{$\lambda$ = 0.2}	& \multicolumn{2}{c|}{$\lambda$ = 0.4}	& \multicolumn{2}{c|}{$\lambda$ = 0.6}	& \multicolumn{2}{c|}{$\lambda$ = 0.8}	& \multicolumn{2}{c|}{$\lambda$ = 1.0} \\ \hline
\textbf{}	& Prec@10	& MAP@10	& Prec@10	& MAP@10	& Prec@10	& MAP@10	& Prec@10	& MAP@10	& Prec@10	& MAP@10	 \\ \hline
Initial	& 0.00419	& 0.00121	& 0.00419	& 0.00121	& 0.00419	& 0.00121	& 0.00419	& 0.00121	& 0.00419	& 0.00121	 \\ \hline
\begin{tabular}[c]{@{}l@{}}Re-ranked\\ Global\end{tabular}	& 0.0033	& 0.00115	& 0.00505	& 0.0012	& \textbf{0.00628}	& 0.00245	& 0.00542	& 0.0029	& 0.00542	& \textbf{0.00291}	 \\ \hline
\begin{tabular}[c]{@{}l@{}}Re-ranked\\ Personal\end{tabular}	& 0.00467	& 0.00276	& 0.00729	& 0.00402	& 0.00901	& 0.00648	& 0.00959	& 0.00783	& \textbf{0.00987}	& \textbf{0.00906}	 \\ \hline
\end{tabular}}
\caption*{Re-rank results for the \textbf{CAMF-ICS} initial recommendation for both global and personal model, evaluated over the \textbf{top 10} songs in the recommendation list consisting of the top \textbf{50 songs} using the \textit{time of day} dimension.}\label{tab:res-CAMF-ICS-50-10}
\end{table}
